# Supplementary material for: Competing phases of HfO$_2$ from unstable flat phonon bands of an unconventional high-symmetry structure
Source: arXiv:2412.16792 ancillary file (2025-07-08)
Supplement: Supplementary file 1 [file Supplementary_Materials_Flat_Band.pdf]

# Supplementary Materials: Understand the specialities and functionalities of $HfO_2$ from unstable flat phonon bands in an unconventional high-symmetry phase

Yubo Qi[1] and Karin M. Rabe[2]

[1]Department of Physics, University of Alabama at Birmingham, Birmingham, Alabama 35233, USA
[2]Department of Physics & Astronomy, Rutgers University, Piscataway, New Jersey 08854, USA

## SECTION 1: THE LATTICE AND COORDINATES

In Table S1 and S2, we show the lattice vectors and atom fractional coordinates of conventional cell and primitive cell for the *Cmma* structure. The conventional cell is a $\sqrt{2} \times \sqrt{2} \times 1$ superlattice of the primitive cell. The unit of the lattice vectors is Å.

| *Cmma* | *x* | *y* | *z* |
|---|---|---|---|
| **a** | 5.15966 | 0.00000 | 0.00000 |
| **b** | 0.00000 | 5.33192 | 0.00000 |
| **c** | 0.00000 | 0.00000 | 4.84891 |
| Hf | 0.25000 | 0.75000 | 0.21215 |
| Hf | 0.75000 | 0.75000 | 0.78785 |
| Hf | 0.25000 | 0.25000 | 0.78785 |
| Hf | 0.75000 | 0.25000 | 0.21215 |
| O | 0.00000 | 0.25000 | 0.50000 |
| O | 0.50000 | 0.25000 | 0.50000 |
| O | 0.50000 | 0.75000 | 0.50000 |
| O | 0.00000 | 0.75000 | 0.50000 |
| O | 0.00000 | 0.50000 | 0.00000 |
| O | 0.50000 | 0.00000 | 0.00000 |
| O | 0.05000 | 0.50000 | 0.00000 |
| O | 0.00000 | 0.00000 | 0.00000 |

TABLE S1. The conventional cell of the *Cmma* structure.

| *Cmma* | *x* | *y* | *z* |
|---|---|---|---|
| **a** | 3.70983 | 0.00000 | 0.00000 |
| **b** | 0.12179 | 3.70783 | 0.00000 |
| **c** | 0.00000 | 0.00000 | 4.84891 |
| Hf | 0.25000 | 0.75000 | 0.78785 |
| Hf | 0.75000 | 0.25000 | 0.21215 |
| O | 0.00000 | 0.00000 | 0.50000 |
| O | 0.50000 | 0.50000 | 0.50000 |
| O | 0.75000 | 0.75000 | 0.00000 |
| O | 0.25000 | 0.25000 | 0.00000 |

TABLE S2. The primitive cell of the *Cmma* structure.

## SECTION 2: COMPUTATIONAL DETAILS

In this work, all density functional theory (DFT) calculations are carried out using the Quantum–espresso [S1] package. The kinetic energy cutoff is 50 Ry, and the the Brillouin zone is sampled by a 4×4×4 Monkhorst–Pack $k$–point mesh [S2]. The convergence threshold on atomic forces for ionic minimization is $1\times10^{-6}$ Hartree per Bohr. Local density approximation (LDA) pseudopotentials are generated by the Opium package [S3, S4]. Here, we would like to emphasize that using a different functional, such as the PBEsol, will also give similar phonon spectrum with 4 unstable flat phonon bands, as in Fig. S1.

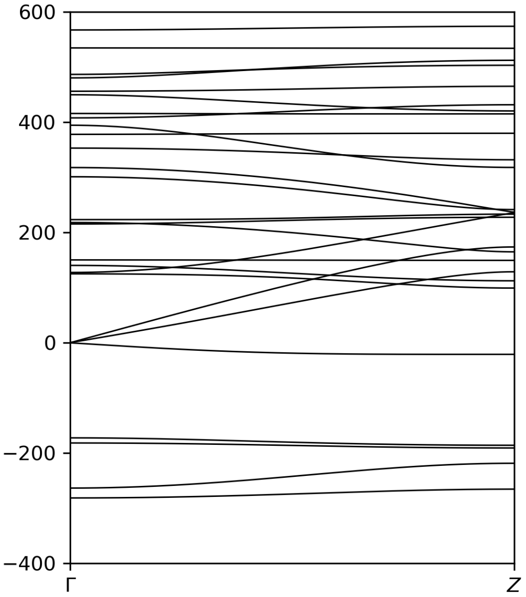


FIG. S1. Phonon spectrum calculated with the PBEsol functional.

## SECTION 3: PHONON SPECTRUM

In this section, we will show the relationship between the phonon spectrum of the primitive cell and that of the conventional cell. The full phonon spectrum of the primitive cell of the $Cmma$ structure is shown in Fig. S2.

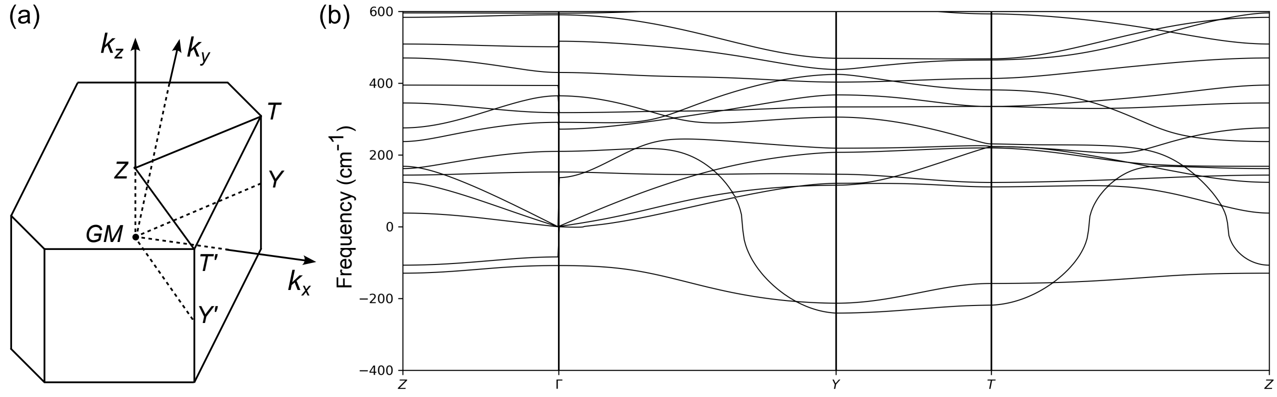


FIG. S2. (a) Brillouin zone and (b) full phonon spectrum of the primitive cell of the $Cmma$ structure.

In Fig. S3 (a), we show the phonon spectrum of the conventional cell along the $\Gamma - Z$ axis, and its relationship with the phonon spectrum of the primitive cell. The phonon bands of conventional cell along the $\Gamma - Z$ axis is the

combination of the phonon bands along the $\Gamma - Z$ axis (indicated by red lines) and he phonon bands along the $Y - T$ axis (indicated by blue lines) of the primitive cell. The labeling of the phonon modes are based on the primitive cell. As shown in Fig. S3 (b), the phonon spectrum of the conventional cell along the $\Gamma - Y$ axis results from folding the phonon bands of the primitive cell with respect to the bisecting central axis along the $\Gamma - Y$ direction. Similarly, as shown in Fig. S3 (c), the phonon spectrum of the conventional cell along the $\Gamma - X$ axis results from folding the phonon bands of the primitive cell with respect to the bisecting central axis along the $\Gamma - Y'$ direction.

Here, there are also unstable phonon bands along the $\Gamma - X$ and $\Gamma - Y$ axes for the conventional cell. Similar to the $\Gamma - Z$ case discussed in the main manuscript, we can also carry out data-driven metastable phase search based on the unstable phonons. The results are shown in section 7 of this supplementary material.

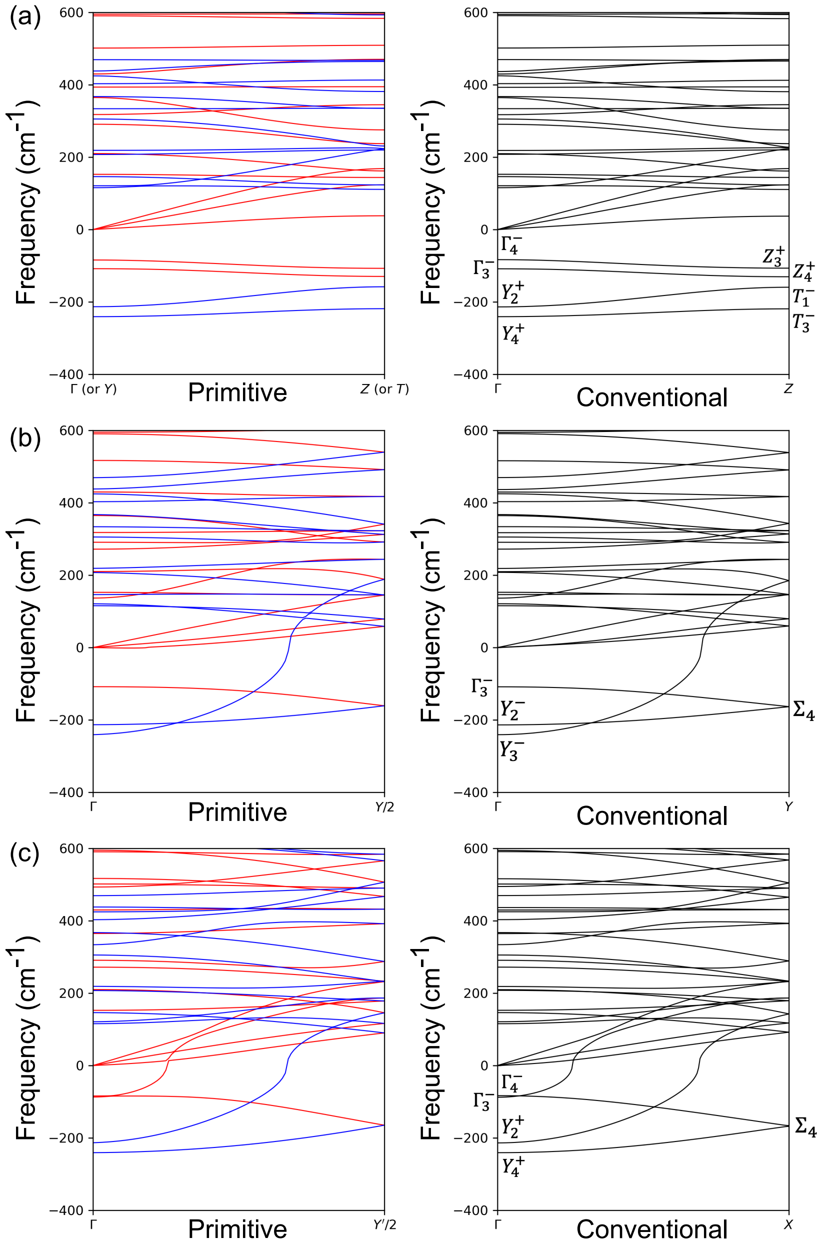


FIG. S3. Relationships between the phonon spectra of the primitive cell and conventional cell along different axes.

## SECTION 4: RELAXED STRUCTURES

In Table S3, we show the optimized structures, with their energies and space groups, relaxed from structures with the activation of different unstable modes, taking the *Cmma* structure as the reference. in Table S4, we show the energies, space groups and mode amplitudes of these structures.

| Zone center mode amplitudes | | | | Zone boundary mode amplitudes | | | | | | |
|---|---|---|---|---|---|---|---|---|---|---|
| $Y_4^+$ | $Y_2^+$ | $\Gamma_3^-$ | $\Gamma_4^-$ | $T_3^-$ | $T_1^-$ | $Z_4^+$ | $Z_3^+$ | Space group | Figure | Energy (meV/f.u.) |
| - | - | - | - | - | - | - | A | $P4_2/nmc$ | Fig. S1 (b) | 80 |
| - | - | - | - | - | A | - | A | | | |
| - | - | - | - | - | A | A | A | | | |
| - | - | - | - | A | - | - | - | | | |
| - | - | - | - | A | - | - | A | | | |
| - | - | - | - | A | A | - | - | | | |
| - | - | - | - | A | A | - | A | | | |
| - | - | - | A | - | - | - | - | | | |
| - | - | - | A | - | - | - | A | | | |
| - | - | - | A | - | - | A | - | | | |
| - | - | - | A | - | A | - | - | | | |
| - | - | - | A | - | A | - | A | | | |
| - | - | - | A | - | A | A | - | | | |
| - | - | - | A | A | - | - | - | | | |
| - | - | - | A | A | - | - | A | | | |
| - | - | - | A | A | - | A | A | | | |
| - | - | - | A | A | A | - | - | | | |
| - | - | A | - | - | - | - | A | | | |
| - | - | A | - | - | - | A | - | | | |
| - | - | A | - | - | A | - | A | | | |
| - | - | A | - | A | - | - | - | | | |
| - | - | A | - | A | - | - | A | | | |
| - | - | A | - | A | A | - | - | | | |
| - | - | A | A | - | A | - | A | | | |
| - | - | A | A | - | A | A | - | | | |
| - | - | A | A | A | - | - | - | | | |
| - | - | A | A | A | A | - | - | | | |
| - | - | A | A | A | A | A | - | | | |
| - | A | A | A | - | A | A | - | | | |
| - | A | A | A | A | - | - | - | | | |
| A | - | - | - | - | - | - | - | | | |
| A | - | - | - | - | - | - | A | | | |
| A | - | - | - | - | - | A | - | | | |
| A | - | - | - | - | A | - | A | | | |
| A | - | - | - | - | A | A | - | | | |
| A | - | - | - | A | - | - | A | | | |
| A | - | - | - | A | - | A | - | | | |
| A | - | - | A | - | - | - | - | | | |
| A | - | - | A | - | - | - | A | | | |
| A | - | - | A | - | - | A | - | | | |
| A | - | - | A | - | A | - | - | | | |
| A | - | - | A | - | A | A | - | | | |
| A | - | - | A | A | - | - | - | | | |
| A | - | - | A | A | - | - | A | | | |
| A | - | - | A | A | A | - | A | | | |
| A | - | - | A | A | A | A | - | | | |
| A | - | - | A | A | A | A | A | | | |
| A | - | A | - | - | A | A | - | | | |
| A | - | A | - | A | A | - | A | | | |
| A | - | A | A | - | A | - | A | | | |
| A | - | A | A | A | - | - | - | | | |
| A | - | A | A | A | - | - | A | | | |
| - | - | - | A | A | A | - | A | $P2_1/c$ | Fig. S1 (c) | 0 |
| - | A | - | - | - | - | - | - | | | |
| - | A | - | - | - | - | A | - | | | |

| | | | | | | | | | | |
|---|---|---|---|---|---|---|---|---|---|---|
| - | A | - | - | - | A | - | - | | | |
| - | A | - | - | - | A | A | - | | | |
| - | A | A | - | - | - | - | - | | | |
| - | A | A | - | - | - | A | - | | | |
| - | A | A | - | - | A | - | - | | | |
| - | A | A | - | A | - | A | A | | | |
| A | - | - | - | - | A | - | - | | | |
| A | - | - | - | A | - | - | - | | | |
| A | - | - | - | A | A | - | - | | | |
| A | - | A | - | A | A | - | - | | | |
| A | A | - | - | - | - | - | - | | | |
| A | A | - | - | - | - | - | A | | | |
| A | A | - | - | - | - | A | - | | | |
| A | A | - | - | - | - | A | A | | | |
| A | A | - | - | - | A | - | - | | | |
| A | A | - | - | - | A | - | A | | | |
| A | A | - | - | - | A | A | - | | | |
| A | A | - | - | A | - | - | - | | | |
| A | A | - | - | A | - | A | - | | | |
| A | A | - | - | A | A | - | - | | | |
| A | A | - | A | - | - | - | - | | | |
| A | A | - | A | - | - | A | - | | | |
| A | A | - | A | - | A | - | - | | | |
| A | A | - | A | - | A | A | - | | | |
| A | A | A | - | - | - | - | - | | | |
| A | A | A | - | - | - | - | A | | | |
| A | A | A | - | - | - | A | - | | | |
| A | A | A | - | - | - | A | A | | | |
| A | A | A | - | - | A | - | - | | | |
| A | A | A | - | - | A | - | A | | | |
| A | A | A | - | - | A | A | - | | | |
| A | A | A | - | A | - | - | - | | | |
| A | A | A | A | - | - | - | - | | | |
| A | A | A | A | - | - | A | - | | | |
| - | - | A | A | - | - | - | - | $Pmn2_1$ | Fig. S1 (d) | 110 |
| - | - | A | A | - | - | - | A | | | |
| - | - | A | A | - | - | A | - | | | |
| - | - | A | A | - | A | - | - | | | |
| A | - | A | - | A | - | - | A | | | |
| A | - | A | A | - | - | - | A | | | |
| - | - | - | A | - | A | A | A | $Pca2_1$ | Fig. S1 (e) | 50 |
| - | - | - | A | A | A | A | A | | | |
| - | - | A | - | - | - | - | - | | | |
| - | - | A | - | A | A | - | A | | | |
| - | - | A | A | A | - | - | A | | | |
| - | - | A | A | A | - | A | A | | | |
| - | - | A | A | A | A | - | A | | | |
| - | - | A | A | A | A | A | A | | | |
| - | A | - | A | - | - | - | - | | | |
| - | A | - | A | - | - | A | - | | | |
| - | A | - | A | - | A | - | - | | | |
| - | A | - | A | - | A | A | - | | | |
| - | A | A | - | - | A | A | - | | | |
| - | A | A | A | - | - | - | - | | | |
| - | A | A | A | - | - | - | A | | | |
| - | A | A | A | - | - | A | - | | | |
| - | A | A | A | - | A | - | - | | | |
| - | A | A | A | A | - | A | A | | | |
| A | - | - | - | A | A | - | A | | | |
| A | - | - | - | A | A | A | A | | | |
| A | - | - | A | A | A | - | - | | | |
| A | - | A | - | - | - | - | - | | | |
| A | - | A | - | - | - | - | A | | | |

| | | | | | | | | | | |
|---|---|---|---|---|---|---|---|---|---|---|
| A | - | A | - | - | - | A | - | | | |
| A | - | A | - | - | - | A | A | | | |
| A | - | A | - | - | A | - | - | | | |
| A | - | A | - | - | A | - | A | | | |
| A | - | A | - | - | A | A | A | | | |
| A | - | A | - | A | - | - | - | | | |
| A | - | A | - | A | - | A | - | | | |
| A | - | A | A | - | - | - | - | | | |
| A | - | A | A | - | - | A | - | | | |
| A | - | A | A | - | A | - | - | | | |
| A | - | A | A | - | A | A | - | | | |
| A | - | A | A | A | - | A | - | | | |
| A | - | A | A | A | - | A | A | | | |
| A | - | A | A | A | A | - | - | | | |
| A | - | A | A | A | A | - | A | | | |
| - | - | - | - | - | - | A | - | *Pbca* | Fig. S1 (f) | 28 |
| - | - | - | - | A | - | A | - | | | |
| - | - | - | - | A | - | A | A | | | |
| - | - | - | - | A | A | A | - | | | |
| - | - | - | - | A | A | A | A | | | |
| - | - | - | A | A | - | A | - | | | |
| - | - | - | A | A | A | A | - | | | |
| - | - | A | - | - | A | A | - | | | |
| - | - | A | - | A | - | A | - | | | |
| - | - | A | - | A | - | A | A | | | |
| - | - | A | A | - | A | A | A | | | |
| - | - | A | A | A | - | A | - | | | |
| - | A | - | - | - | - | - | A | | | |
| - | A | - | - | - | - | A | A | | | |
| - | A | - | - | - | A | - | A | | | |
| - | A | - | - | - | A | A | A | | | |
| - | A | - | A | - | - | A | A | | | |
| - | A | - | A | - | A | A | A | | | |
| - | A | A | - | - | - | - | A | | | |
| - | A | A | - | - | - | A | A | | | |
| - | A | A | - | - | A | - | A | | | |
| - | A | A | A | - | - | A | A | | | |
| A | - | - | - | A | A | A | - | | | |
| A | - | - | A | - | - | A | A | | | |
| A | - | - | A | - | A | A | A | | | |
| A | - | A | - | A | - | A | A | | | |
| A | - | A | - | A | A | A | - | | | |
| A | - | A | A | - | - | A | A | | | |
| A | A | - | - | A | A | A | - | | | |
| A | A | A | - | A | - | A | - | | | |
| A | A | A | - | A | A | - | - | | | |
| A | A | A | - | A | A | A | - | | | |
| A | A | A | A | - | A | A | - | | | |
| - | - | - | - | - | A | A | - | *Pc* | Fig. 3 (a) | 39 |
| - | - | A | - | - | A | - | - | | | |
| - | A | - | - | A | - | - | A | | | |
| - | A | - | - | A | - | A | A | | | |
| - | A | - | - | A | A | - | A | | | |
| - | A | - | A | - | - | - | A | | | |
| - | A | - | A | - | A | - | A | | | |
| - | A | - | A | A | - | - | - | | | |
| - | A | - | A | A | - | - | A | | | |
| - | A | - | A | A | - | A | A | | | |
| - | A | - | A | A | A | - | - | | | |
| - | A | - | A | A | A | - | A | | | |
| - | A | - | A | A | A | A | - | | | |
| - | A | A | A | - | A | - | A | | | |
| - | A | A | A | A | - | - | A | | | |

| | | | | | | | | | | |
|---|---|---|---|---|---|---|---|---|---|---|
| - | A | A | A | A | - | A | - | | | |
| - | A | A | A | A | A | - | - | | | |
| A | - | - | A | - | A | - | A | | | |
| A | - | A | A | - | A | A | A | | | |
| A | A | - | - | - | A | A | A | | | |
| A | A | - | - | A | - | - | A | | | |
| A | A | - | - | A | - | A | A | | | |
| A | A | - | - | A | A | - | A | | | |
| A | A | - | - | A | A | A | A | | | |
| A | A | - | A | - | - | - | A | | | |
| A | A | - | A | - | - | A | A | | | |
| A | A | - | A | - | A | - | A | | | |
| A | A | - | A | A | - | - | - | | | |
| A | A | - | A | A | - | - | A | | | |
| A | A | - | A | A | - | A | - | | | |
| A | A | - | A | A | - | A | A | | | |
| A | A | - | A | A | A | - | - | | | |
| A | A | - | A | A | A | - | A | | | |
| A | A | - | A | A | A | A | - | | | |
| A | A | A | - | A | - | - | A | | | |
| A | A | A | - | A | A | - | A | | | |
| A | A | A | A | - | - | - | A | | | |
| A | A | A | A | - | A | - | - | | | |
| A | A | A | A | A | - | - | - | | | |
| A | A | A | A | A | - | - | A | | | |
| A | A | A | A | A | A | - | - | | | |
| - | - | A | - | A | A | A | A | *Pbca* | Fig. 3 (b) | 27 |
| - | A | - | - | A | - | - | - | | | |
| - | A | - | - | A | - | A | - | | | |
| - | A | - | - | A | A | - | - | | | |
| - | A | - | - | A | A | A | - | | | |
| - | A | - | A | A | - | A | - | | | |
| - | A | A | - | A | - | - | - | | | |
| - | A | A | - | A | - | - | A | | | |
| - | A | A | - | A | - | A | - | | | |
| - | A | A | - | A | A | - | - | | | |
| - | A | A | - | A | A | A | - | | | |
| - | - | - | - | - | A | - | - | $C2/c$ | Fig. 3 (c) | 385 |
| - | A | - | - | A | A | A | A | $Cc$ | Fig. 3 (d) | 179 |
| - | A | - | A | A | A | A | A | | | |
| - | A | A | - | A | A | - | A | | | |
| - | A | A | - | A | A | A | A | | | |
| - | A | A | A | - | A | A | A | | | |
| - | A | A | A | A | A | - | A | | | |
| - | A | A | A | A | A | A | - | | | |
| - | A | A | A | A | A | A | A | | | |
| A | - | A | - | A | A | A | A | | | |
| A | - | A | A | A | A | A | - | | | |
| A | - | A | A | A | A | A | A | | | |
| A | A | - | A | - | A | A | A | | | |
| A | A | - | A | A | A | A | A | | | |
| A | A | A | - | - | A | A | A | | | |
| A | A | A | - | A | - | A | A | | | |
| A | A | A | - | A | A | A | A | | | |
| A | A | A | A | - | - | A | A | | | |
| A | A | A | A | - | A | - | A | | | |
| A | A | A | A | - | A | A | A | | | |
| A | A | A | A | A | - | A | - | | | |
| A | A | A | A | A | - | A | A | | | |
| A | A | A | A | A | A | - | A | | | |
| A | A | A | A | A | A | A | - | | | |
| A | A | A | A | A | A | A | A | | | |
| - | - | A | - | A | A | A | - | $P2_1$ | Fig. 3 (e) | 206 |

| | | | | | | | | | | |
|---|---|---|---|---|---|---|---|---|---|---|
| - | - | - | - | - | - | A | A | *Pnma* | Fig. 3 (f) | 97 |
| - | - | - | A | - | - | A | A | | | |
| - | - | A | - | - | - | A | A | | | |
| - | - | A | - | - | A | A | A | | | |
| - | - | A | A | - | - | A | A | | | |
| - | A | A | - | - | A | A | A | | | |
| A | - | - | - | A | - | A | A | | | |
| A | - | - | A | A | - | A | - | | | |
| A | - | - | A | A | - | A | A | | | |
| A | - | - | - | - | - | A | A | $P2_1/c$ | Fig. 3 (g) | 79 |
| A | - | - | - | - | A | A | A | | | |

TABLE S3: Structures, with their energies and space groups, optimized from structures with the activation of different unstable modes.

| | | | Branch 1 | | Branch 2 | | Branch 3 | | Branch 4 | |
|---|---|---|---|---|---|---|---|---|---|---|
| Space group | Figure | Energy (meV/f.u.) | $Y_4^+$ | $T_3^-$ | $Y_2^+$ | $T_1^-$ | $\Gamma_3^-$ | $Z_4^+$ | $\Gamma_4^-$ | $Z_3^+$ |
| $P4_2/nmc$ | Fig. 3 (a) | 80 | 0 | 0 | 0.08 | 0 | 0 | 0 | 0.62 | 0 |
| $P2_1/c$ | Fig. 3 (b) | 0 | 0.20 | 0 | -0.27 | 0 | 0 | 0 | 0 | 0 |
| $Pmn2_1$ | Fig. 3 (c) | 110 | 0 | 0 | 0 | 0 | 0.24 | 0 | 0.43 | 0 |
| $Pca2_1$ | Fig. 3 (d) | 50 | 0 | 0 | 0.30 | 0 | 0 | 0 | 0.33 | 0 |
| *Pbca* | Fig. 3 (e) | 28 | 0 | 0 | 0.32 | 0 | 0 | 0 | 0 | 0.31 |
| *Pbca* | Fig. 3 (f) | 27 | 0 | 0.20 | 0.22 | 0 | 0 | 0 | 0 | 0 |
| $C2/c$ | Fig. 3 (g) | 385 | 0 | 0.14 | 0 | 0.30 | 0 | 0 | 0 | 0 |
| *Pc* | Fig. 3 (h) | 39 | 0.09 | -0.07 | 0.30 | 0 | 0 | 0 | -0.16 | 0.16 |
| *Cc* | Fig. 3 (i) | 179 | 0.18 | 0.18 | 0.14 | 0.12 | 0.13 | 0.14 | 0.20 | 0.20 |
| $P2_1$ | Fig. 3 (j) | 206 | 0 | 0.34 | 0.05 | 0 | 0.13 | 0.17 | 0 | 0 |
| *Pnma* | Fig. 3 (k) | 97 | 0 | 0 | 0 | 0 | 0 | 0.25 | 0 | 0.41 |
| $P2_1/c$ | Fig. 3 (l) | 79 | 0.16 | -0.32 | 0 | 0 | -0.03 | 0.12 | 0.33 | -0.20 |

TABLE S4. The space groups, energies, and amplitudes of the unstable modes of the discovered structures. In each branch, the mode at left is the zone center mode, and the one at right is the zone boundary mode. Modes amplitudes larger than 0.02 Å are reported.

## SECTION 5: PHONON SPECTRA OF THE UNCONVENTIONAL STRUCTURES

In this section, we shown the phonon spectra of the 7 unconventional structures [structures in Fig. 3 (f-l)] discovered through phonon-mode-inspired high throughput search. Their phonon spectra indicate that all these phases are stable.

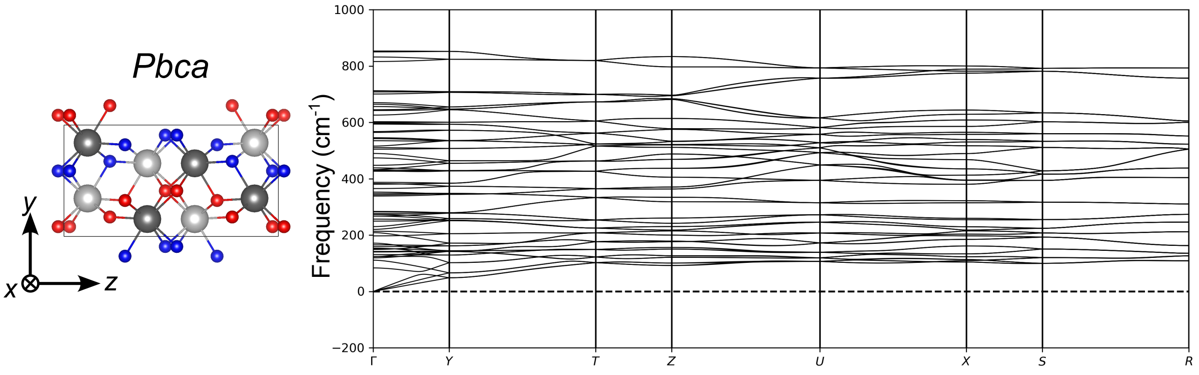


FIG. S4. The phonon spectrum of the *Pbca* structure in Fig. 3 (f).

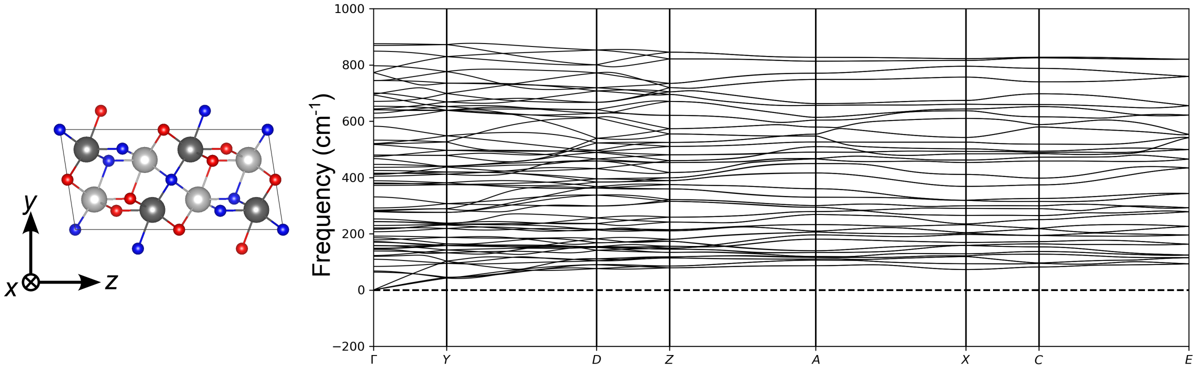


FIG. S5. The phonon spectrum of the $C2/c$ structure in Fig. 3 (g).

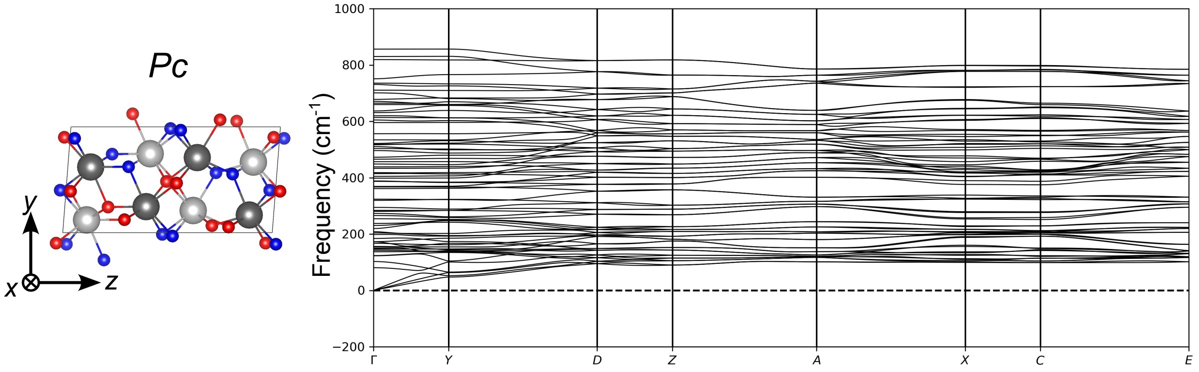


FIG. S6. The phonon spectrum of the $Pc$ structure in Fig. 3 (h).

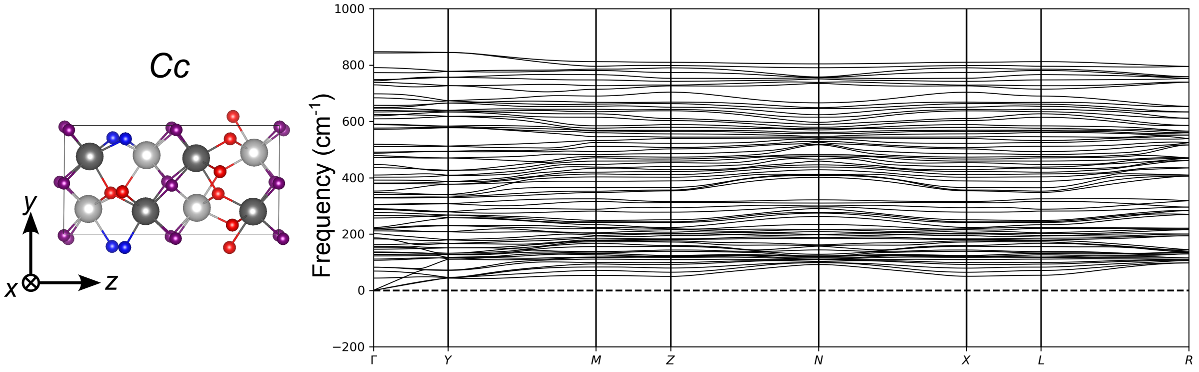


FIG. S7. The phonon spectrum of the $Cc$ structure in Fig. 3 (i).

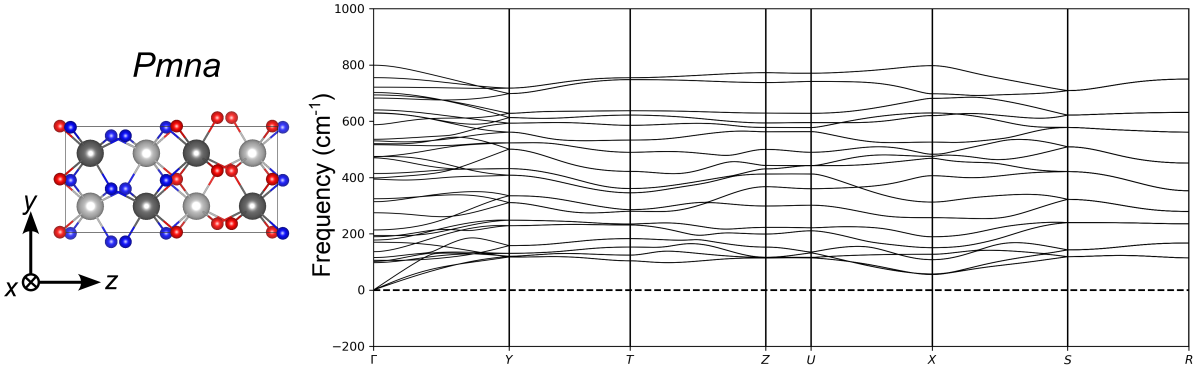


FIG. S8. The phonon spectrum of the *Pmna* structure in Fig. 3 (j).

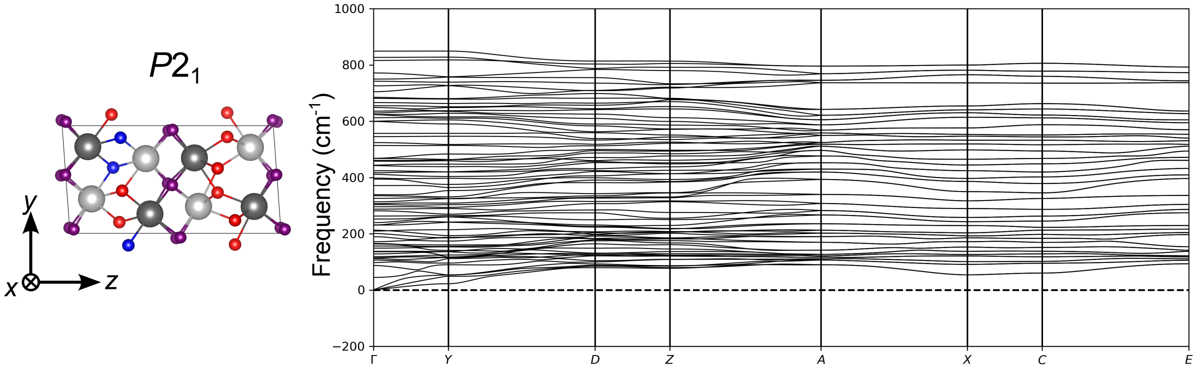


FIG. S9. The phonon spectrum of the $P2_1$ structure in Fig. 3 (k).

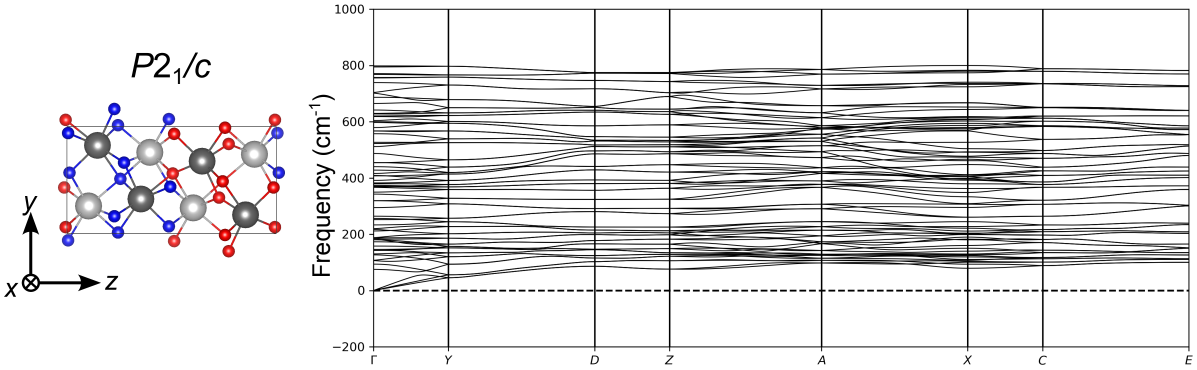


FIG. S10. The phonon spectrum of the $P2_1/c$ structure in Fig. 3 (l).

## SECTION 6: ACTIVATION OF MODES IN SUPERLATTICES

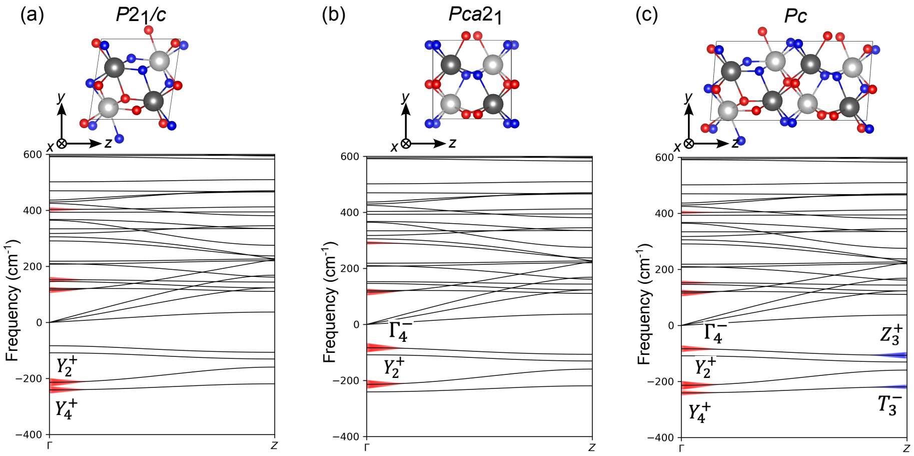


FIG. S11. Activation and softening of the phonon modes for the (a) m $P2_1/c$, (b) o-FE $Pca2_1$, and (c) $Pc$ structures.

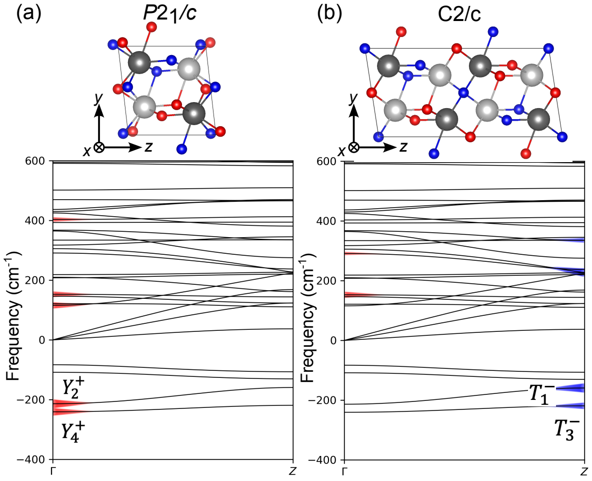


FIG. S12. Activation and softening of the phonon modes for the (a) m $P2_1/c$ and (b) $C2/c$ structures. The $C2/c$ structures is also shown in Fig. 3 (g).

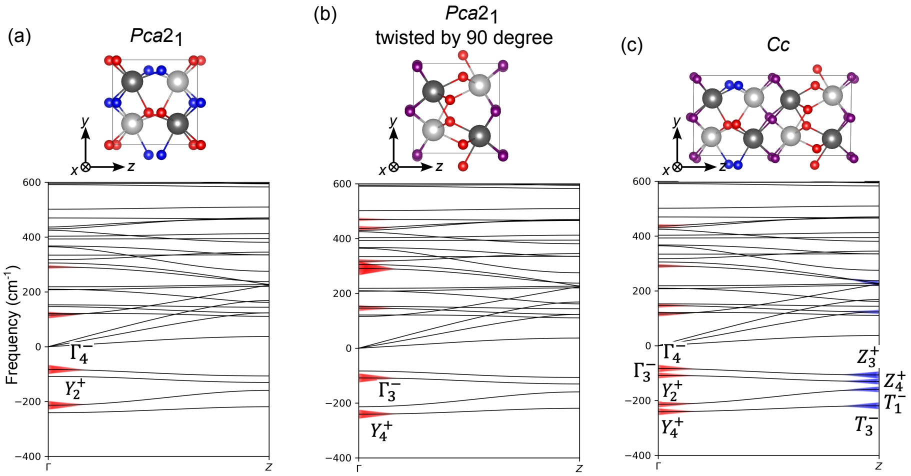


FIG. S13. Activation and softening of the phonon modes for the (a) o-FE $Pca2_1/c$ structure, (b) o-FE $Pca2_1/c$ structure twisted by 90°, and (c) $Cc$ structure. The $Cc$ structures is also shown in Fig. 3 (i).

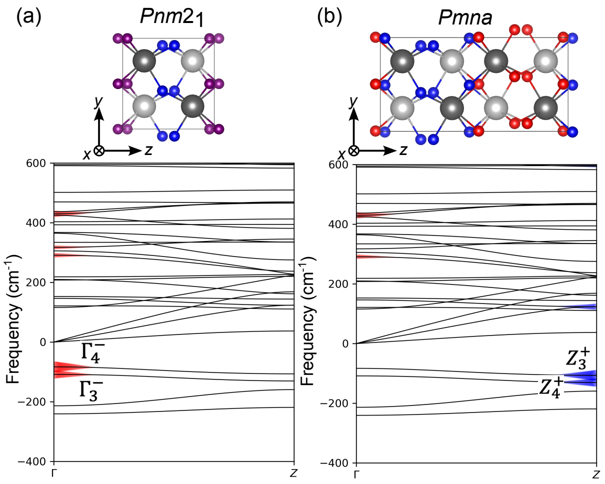


FIG. S14. Activation and softening of the phonon modes for the (a) o-FE2 $Pnm2_1/c$ and (b) $Pmna$ structures. The $Pmna$ structures is also shown in Fig. 3 (j).

## SECTION 7: OTHER DISCOVERED STRUCTURES

In this section, we show the superlattices/phases discovered using the unstable modes along the $\Gamma - X$ axis. There are 6 unstable modes, leading to $2^6 = 64$ different initial configurations. After relaxing these $2^6 = 64$ structures, we acquired 4 new phases. Their space groups, energies, and mode amplitudes are summarized in Table S5 and their structures are shown in Fig. S15. The relaxed structures under the activations of different unstable modes are shown in Table S6.

No new structures are discovered based on analysis along the $\Gamma - Y$ axis.

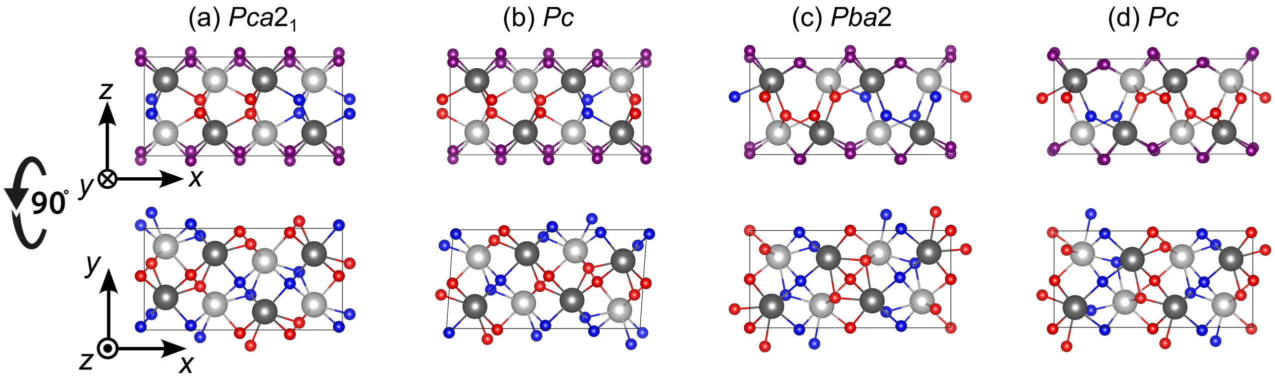


FIG. S15. The other superlattices/phases discovered using the unstable modes along the $\Gamma - X$ axis.

| | | | Zone center | | | | Zone boundary | |
|---|---|---|---|---|---|---|---|---|
| Space group | Figure | Energy (meV/f.u.) | $Y_4^+$ | $Y_2^+$ | $\Gamma_3^-$ | $\Gamma_4^-$ | $\Sigma_4$ (1) | $\Sigma_4$ (2) |
| $Pca2_1$ | Fig. S4 (a) | 95 | 0 | 0 | 0.29 | 0 | -0.23 | 0.25 |
| $Pc$ | Fig. S4 (b) | 92 | -0.17 | 0 | -0.28 | 0.20 | -0.01 | 0.24 |
| $Pba2$ | Fig. S4 (c) | 134 | 0 | 0.38 | 0 | 0 | 0 | 0.19 |
| $Pc$ | Fig. S4 (d) | 103 | -0.07 | 0.33 | 0 | 0.16 | 0 | -0.17 |

TABLE S5: The discovered structures, their amplitudes of the unstable modes, energies, and space groups.

| Zone center | | | | Zone boundary | | | | |
|---|---|---|---|---|---|---|---|---|
| $Y_4^+$ | $Y_2^+$ | $\Gamma_3^-$ | $\Gamma_4^-$ | $\Sigma_4$ (1) | $\Sigma_4$ (2) | Space group | Figure | Energy (meV/f.u.) |
| - | - | - | - | - | A | $P4_2/nmc$ | Fig. S1 (b) | 80 |
| - | - | - | - | A | - | | | |
| - | - | - | - | A | A | | | |
| - | - | - | - | A | A | | | |
| - | A | - | - | - | - | | | |
| - | A | - | - | - | - | | | |
| - | A | - | - | - | A | | | |
| - | A | - | - | - | A | | | |
| - | A | - | - | A | - | | | |
| - | A | - | - | A | - | | | |
| - | A | - | - | A | A | | | |
| - | A | - | - | A | A | | | |
| - | A | A | A | A | A | | | |
| - | - | - | - | - | - | $P2_1/c$ | Fig. S1 (c) | 0 |
| - | - | - | - | - | - | | | |
| - | - | A | A | - | - | | | |
| - | - | A | A | - | - | | | |
| - | - | A | A | A | A | | | |
| - | A | A | - | - | - | | | |
| - | A | A | - | - | - | | | |
| - | A | A | - | - | A | | | |
| - | A | A | - | - | A | | | |

| | | | | | | | | |
|---|---|---|---|---|---|---|---|---|
| - | A | A | - | A | - | | | |
| - | A | A | - | A | - | | | |
| - | A | A | A | - | - | | | |
| - | A | A | A | - | - | | | |
| - | A | A | A | - | A | | | |
| - | A | A | A | - | A | | | |
| - | A | A | A | A | - | | | |
| - | A | A | A | A | - | | | |
| - | A | A | A | A | A | | | |
| - | - | - | - | A | - | $Pca2_1$ | Fig. S1 (e) | 50 |
| - | - | - | A | - | - | | | |
| - | - | - | A | - | - | | | |
| - | - | A | - | A | - | | | |
| - | - | A | - | A | - | | | |
| - | - | A | A | A | - | | | |
| - | - | A | A | A | - | | | |
| - | A | - | A | - | - | | | |
| - | A | - | A | - | - | | | |
| - | A | - | A | - | A | | | |
| - | A | - | A | - | A | | | |
| - | A | - | A | A | - | | | |
| - | A | - | A | A | - | | | |
| - | - | - | A | A | - | $Pmn2_1$ | Fig. S1 (d) | 110 |
| - | - | - | A | A | - | | | |
| - | - | - | - | - | A | $Pca2_1$ | Fig. S4 (a) | 95 |
| - | - | - | A | - | A | | | |
| - | - | - | A | - | A | | | |
| - | - | - | A | A | A | $Pc$ | Fig. S4 (b) | 92 |
| - | - | - | A | A | A | | | |
| - | A | - | A | A | A | | | |
| - | A | - | A | A | A | | | |
| - | - | A | - | - | - | $Pba2$ | Fig. S4 (c) | 134 |
| - | - | A | - | - | A | | | |
| - | - | A | - | - | A | | | |
| - | - | A | A | - | A | | | |
| - | - | A | - | - | - | $Pc$ | Fig. S4 (d) | 103 |
| - | - | A | - | A | A | | | |
| - | - | A | - | A | A | | | |
| - | - | A | A | - | A | | | |
| - | - | A | A | A | A | | | |
| - | A | A | - | A | A | | | |
| - | A | A | - | A | A | | | |

TABLE S6: Structures, with their energies and space groups, optimized from structures with the activations of different unstable modes.


[S1] P. Giannozzi, S. Baroni, N. Bonini, M. Calandra, R. Car, C. Cavazzoni, D. Ceresoli, G. L. Chiarotti, M. Cococcioni, I. Dabo, A. D. Corso, S. de Gironcoli, S. Fabris, G. Fratesi, R. Gebauer, U. Gerstmann, C. Gougoussis, A. Kokalj, M. Lazzeri, L. Martin-Samos, N. Marzari, F. Mauri, R. Mazzarello, S. Paolini, A. Pasquarello, L. Paulatto, C. Sbraccia, S. Scandolo, G. Sclauzero, A. P. Seitsonen, A. Smogunov, P. Umari, and R. M. Wentzcovitch, Quantum espresso: A modular and open-source software project for quantum simulations of materials, Journal of Physics: Condensed Matter **21**, 395502 (2009).

[S2] H. J. Monkhorst and J. D. Pack, Special points for brillouin-zone integrations, Physical Review B **13**, 5188 (1976).

[S3] http://opium.sourceforge.net.

[S4] J. W. Bennett, Discovery and design of functional materials: integration of database searching and first principles calculations, Physics Procedia **34**, 14 (2012).
